# Supplementary material for: Exploring the limits of strong membership inference attacks on large language models
Source: arXiv:2505.18773 source file (2026-01-08)
Supplement: Supplementary file 1 [file appendix.tex]

\section{RMIA investigation}

\section{Some examples that are vulnerable / not vulnerable}

smallest but in, largest but out, difficult examples etc.
