# Supplementary material for: Exploring the limits of strong membership inference attacks on large language models
Source: arXiv:2505.18773 source file (2026-01-08)
Supplement: Supplementary file 2 [file 99_unused_mia_background.tex]

\section{Extended Background on Membership Inference}
\label{app:background}

A membership inference attack (MIA)~\citep{shokri2017membership}, given a model $f_{\theta_T}(x)$ and a data point $x\in D_T$ from a target dataset $D_T$ aims to infer whether the model was trained on $x$.

\subsection{Likelihood Ratio Attack}
\citet{carlini2022membership} propose the Likelihood Ratio Attack (LiRA), which treats membership inference as a hypothesis test. They argue that an effective MIA must have a high true positive rate (TPR) at a low false positive rate (FPR). 

\paragraph{The Offline Attack.}
The intuition behind the offline version of the attack is that if $x \in D_T$, then $f_{\theta_T}(x)$ will likely be higher than $f_\theta(x)$ for models $\theta$ not trained on $x$. This means, the model will be more confident with its prediction on $x$. Formally, the attacker assumes the null hypothesis that $x \notin D_T$ and uses the observed $f_{\theta_T}(x)$ to decide whether to reject it.

Concretely, the attacker estimates the conditional probability:
\[
S(x, \theta_T) = \Pr_{\theta, D} \left[ f_\theta(x) \leq f_{\theta_T}(x) \mid x \notin D \right]
\]
where $\theta$ is trained on a shadow dataset $D \sim \mathcal{D}$. To model this distribution, the attacker computes $f_i(x)$ using shadow models $\theta_i$ trained on $D_i$ such that $x \notin D_i$. 

The authors of LiRA assume the logits of $f_i(x)$ follow a normal distribution, and use these samples to estimate the mean and variance of a Gaussian distribution, which is then used to estimate the cumulative distribution function above.
Since LiRA emphasizes the importance of controlling the $\mathrm{FPR}$ $\alpha$, then the threshold $\tau$ for classification becomes $\tau = 1 - \alpha$, treating $\alpha$ as the significance level of a one-tailed hypothesis test.

\paragraph{The Online Attack.}
In the online variant, the membership score is defined as a likelihood ratio:
\[
S(x, \theta_T) = \frac{p_{\theta, D}(f_{\theta_T}(x) \mid x \in D)}{p_{\theta, D}(f_{\theta_T}(x) \mid x \notin D)}
\]
Here, $p_{\theta, D}$ denotes a probability density over $f_\theta(x)$ induced by sampling both $\theta$ and $D$.

In the same vein as in the offline variant, the outputs of $f_\theta(x)$ are assumed to be normally distributed. However, now the attacker trains two sets of shadow models: $\theta^{\text{out}}_i$ on $D^{\text{out}}_i = D_i \setminus \{x\}$ and $\theta^{\text{in}}_i$ on $D^{\text{in}}_i = D_i \cup \{x\}$. The attacker fits Gaussians to the resulting sets of $f_\theta(x)$ values to estimate the numerator and denominator of the membership score.

The intuition here is that there are two possible possibilities: 1) $x \in D_T$ and 2) $x \notin D_T$. The attacker infers which one is true by understanding how likely the observed $f_{\theta_T}(x)$ is under each modeled distribution.
Due to the necessity of training a fresh set of shadow models for every data point $x$, the online attack is computationally significantly more expensive than the offline variant.

\subsection{Robust Membership Inference Attack}

LiRA relies on the fact that a good membership score $S(x, \theta_T)$ should be higher than $S(x, \theta)$ for most shadow models $\theta$. \citet{zarifzadehlow} extend this and propose proposing that $S(x, \theta_T)$ should also exceed $S(z, \theta_T)$ for most $z \sim \mathcal{D}$. In their RMIA, if $x \in D_T$, then $\Pr(\theta_T \mid x \in D_T)$ should exceed $\Pr(\theta_T \mid z \in D_T)$ for random $z$.

Here, $f_\theta(x)$ can be treated as a probability distribution $p(x \mid \theta)$, enabling use of Bayes' Theorem. The attacker estimates the prior using shadow models $\theta_i$:
\[
p(x) = \sum_{\theta' \in \mathcal{M}} p(x \mid \theta') p(\theta') \approx \frac{1}{N} \sum_{i=1}^N f_i(x)
\]


To compute the likelihood ratio of $\theta_T$ between $x$ and $z$, the attacker calculates:
\[
\text{LR}_{\theta_T}(x, z) = \frac{p_\theta(\theta_T \mid x)}{p_\theta(\theta_T \mid z)} = 
\left( \frac{p(x \mid \theta_T)}{p(x)} \right) \cdot \left( \frac{p(z \mid \theta_T)}{p(z)} \right)^{-1}
= \left( \frac{f_{\theta_T}(x)}{p(x)} \right) \cdot \left( \frac{f_{\theta_T}(z)}{p(z)} \right)^{-1}
\]

Finally, by sampling $z_j \sim \mathcal{D}$ for $j \in [M]$, the attacker defines the membership score as
\[
S(x, \theta_T) = \Pr_{z}[\text{LR}_{\theta_T}(x, z) \geq \gamma] \approx \frac{1}{M} \sum_{i=1}^M \mathbbm{1} [\text{LR}_{\theta_T}(x, z_i) \geq \gamma],
\]

where $\gamma$ is a hyperparamter. 
